# Supplementary material for: The Li-F-H Ternary System at High Pressures
Source: arXiv:2012.15336 source file (2020-12-30)
Supplement: Supplementary file 1 [file LiFHn-SI.pdf]

# Supplemental Information for "The Li-F-H Ternary System at High Pressures"

Tiange Bi[1], Andrew Shamp[1], Tyson Terpstra[1], Russell J. Hemley[3], and Eva Zurek[1]

[1]Department of Chemistry, State University of New York at Buffalo, Buffalo, NY 14260-3000, USA]
[3]Departments of Physics and Chemistry, University of Illinois at Chicago, Chicago, Illinois 60607, USA

December 23, 2020

# Contents

**S1 POTCAR Test** **3**

**S2 Convergence Test** **4**

**S3 3D Convex Hull of Li-H-F Phases at 300 GPa** **5**

**S4 Relative Enthalpy Plot for $LiFH_2$ Phases** **9**

**S5 Structural Coordinates of Li-F-H Phases at 300 GPa** **10**

**S6 Structural Coordinates of the Reference Phases at 300 GPa** **18**

**S7 Bader Analysis at 300 GPa** **20**

**S8 Electron Localization Function (ELF) Calculated for $LiF_3H_2$, $LiF_2H$ and $LiF_4H_4$** **21**

**S9 Phonon DOS of Li-F-H Phases at 300 GPa** **24**

**S10 Infrared (IR) Spectra of HF and Li-F-H Phases at 300 GPa** **31**

# S1 POTCAR Test

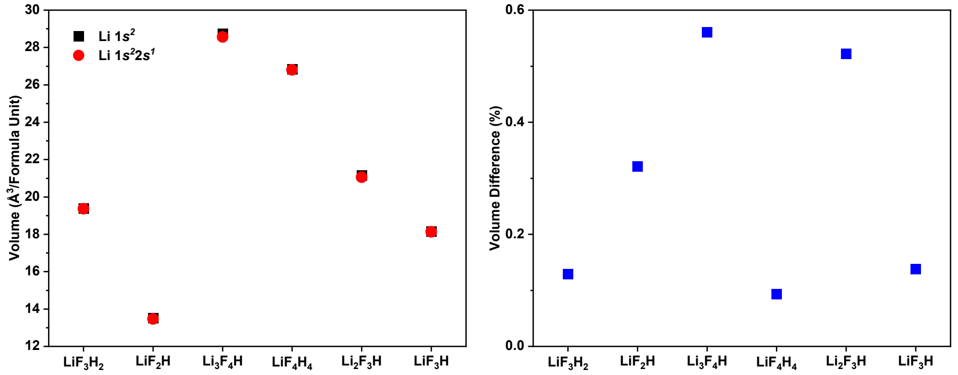


Figure S1: A comparison of the results obtained from structure optimizations carried out using different Li POTCARs at 300 GPa. (Left) Volume of the five lowest enthalpy structures calculated using both the Li $2s^1$ and the Li $1s^2 2s^1$ POTCARs; (Right) percent volume difference obtained via $\frac{a-b}{b} \times 100\%$, where $a$ and $b$ are the volumes calculated using the Li $2s^1$ and the Li $1s^2 2s^1$ POTCARs, respectively. The purpose of this test is to confirm the transferrability of the crystal structure prediction results. The Li $2s^1$ POTCAR is used in the searches, and the Li $1s^2 2s^1$ POTCAR is used otherwise. The maximum $\%$ volume difference is $0.56\%$, suggesting that switching the POTCAR does not influence the results of calculations for the ternary hydrides.

## S2 Convergence Test

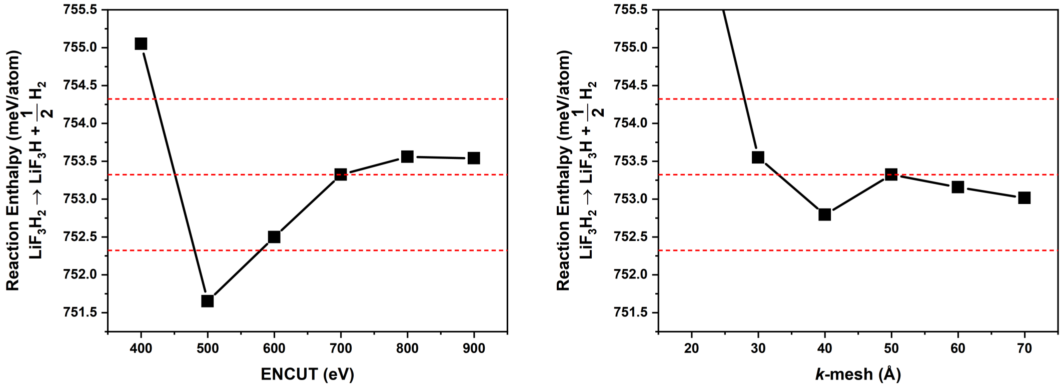


Figure S2: Enthalpy change of the reaction, $LiF_3H_2 \rightarrow LiF_3H + \frac{1}{2}H_2$, at 300 GPa as a function of (left) the cutoff energy used in the plane wave basis set (ENCUT) with the $k$-point grids generated so the number of divisions along each reciprocal lattice vector was chosen such that the product of this number with the real lattice constant was 50 Å, and (b) the product of divisions along each reciprocal lattice vector with the real lattice constant with an ENCUT of 700 eV employed for all calculations.

## S3 3D Convex Hull of Li-H-F Phases at 300 GPa

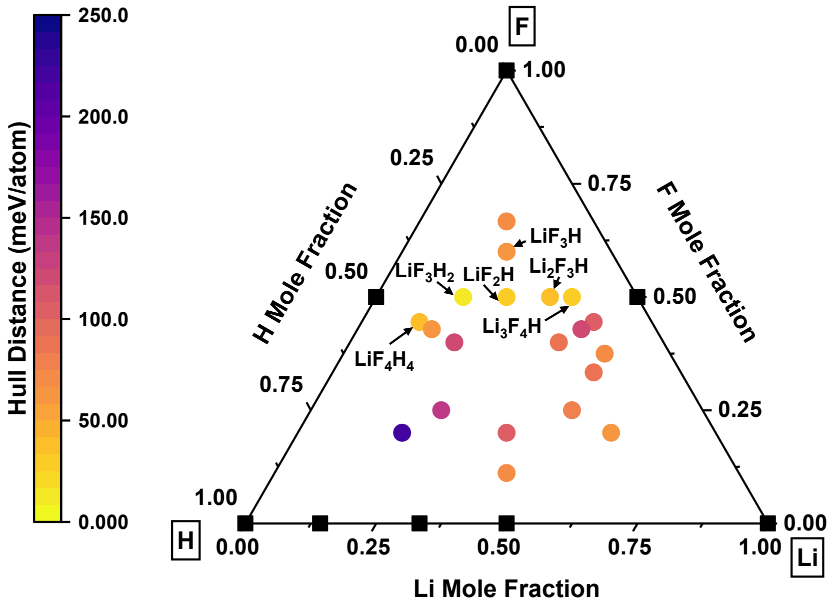


Figure S3: Ternary Li-H-F phase diagram at 300 GPa and 0 K. The data points are colored according to their distance from the convex hull, in meV/atom. Squares represent thermodynamically stable phases, and circles represent metastable phases. Black lines connect stable phases. The hull distance was calculated using the enthalpies of the following experimentally determined or theoretically predicted structures: $P4_2/mbc$ phase of Li,[1] $Cmca$-12 phase of $H_2$,[2] $Cmca$ phase of $F_2$,[3] $Fm\bar{3}m$ phase of LiF,[4,5] $Pnma$ phase of HF,[6–8] $Pm\bar{3}m$ phase of LiH,[9] $P4/mbm$ phase of $LiH_2$, and $R\bar{3}m$ phase of $LiH_6$.[10]

Table S1: The number of atoms of Li, F, and H within one formula unit, and the distance above the convex hull in meV/atom for each phase at 300 GPa and 0 K.

| Li | F | H | Distance above the hull (meV/atom) |
|---|---|---|---|
| 1 | 3 | 2 | 13.3 |
| 1 | 2 | 1 | 29.3 |
| 3 | 4 | 1 | 33.1 |
| 1 | 4 | 4 | 33.4 |
| 2 | 3 | 1 | 40.5 |
| 1 | 3 | 3 | 58.5 |
| 3 | 1 | 1 | 61.9 |
| 1 | 3 | 1 | 62.5 |
| 4 | 3 | 1 | 68.9 |
| 4 | 1 | 4 | 73.4 |
| 1 | 4 | 1 | 74.1 |
| 2 | 1 | 1 | 81.7 |
| 2 | 2 | 1 | 85.1 |
| 3 | 2 | 1 | 90.1 |
| 4 | 4 | 1 | 102.5 |
| 2 | 1 | 2 | 107.5 |
| 1 | 2 | 2 | 118.9 |
| 3 | 3 | 1 | 124.4 |
| 1 | 1 | 2 | 139.5 |
| 1 | 1 | 3 | 222.5 |

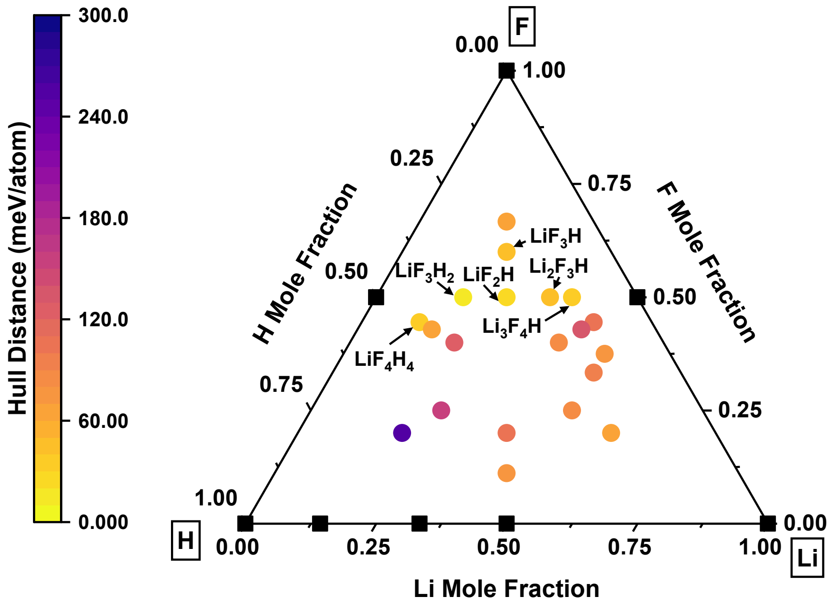


Figure S4: Same as Fig. S3, but the zero-point-energy (ZPE) was taken into consideration.

Table S2: The number of atoms of Li, F, and H within one formula unit, and the distance above the convex hull in meV/atom for each phase at 300 GPa and 0 K including the ZPE.

| Li | F | H | Distance above the hull (meV/atom) |
|---|---|---|---|
| 1 | 3 | 2 | 10.9 |
| 1 | 2 | 1 | 28.5 |
| 3 | 4 | 1 | 33.8 |
| 1 | 4 | 4 | 37.0 |
| 2 | 3 | 1 | 41.1 |
| 1 | 3 | 1 | 49.0 |
| 1 | 3 | 3 | 61.4 |
| 3 | 1 | 1 | 64.1 |
| 1 | 4 | 1 | 68.4 |
| 4 | 1 | 4 | 73.2 |
| 4 | 3 | 1 | 74.1 |
| 2 | 2 | 1 | 85.4 |
| 2 | 1 | 1 | 89.2 |
| 3 | 2 | 1 | 96.9 |
| 4 | 4 | 1 | 106.5 |
| 2 | 1 | 2 | 106.8 |
| 1 | 2 | 2 | 129.2 |
| 3 | 3 | 1 | 131.1 |
| 1 | 1 | 2 | 157.8 |
| 1 | 1 | 3 | 257.7 |

## S4 Relative Enthalpy Plot for $LiFH_2$ Phases

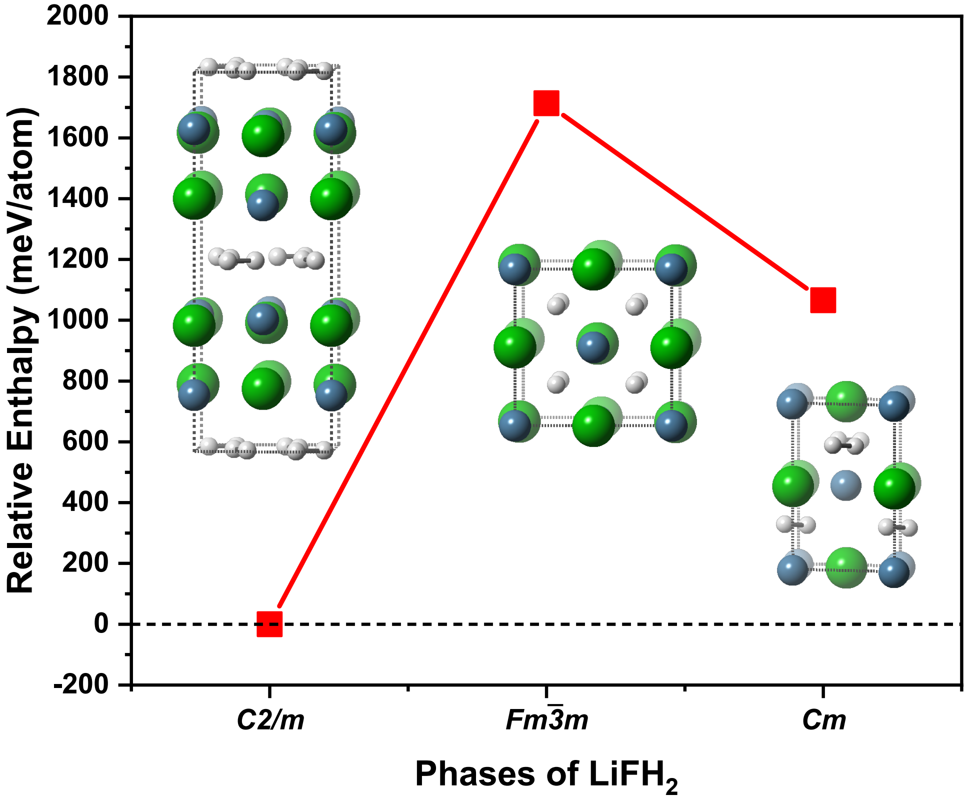


Figure S5: The relative enthalpy plot for the $C2/m$, $Fm\bar{3}m$, and $Cm$ $LiFH_2$ phases with respect to the enthalpy of the $C2/m$ phase. In the structure figures, Li/F/H are colored blue/green/white. The $Fm\bar{3}m$ phase with atomic hydrogen and the $Cm$ phase with molecular hydrogen were proposed by Gilman.[11] Both of the phases are optimized at 300 GPa, and are less stable compared to the $C2/m$ phase found in the evolutionary search.

# S5 Structural Coordinates of Li-F-H Phases at 300 GPa

| $LiFH_2$ | $C2/m$ |
|---|---|
| a, b, c (Å) | 3.122 8.652 3.122 |
| $\alpha, \beta, \gamma$ (Θ) | 90.00 90.00 90.00 |
| F (4h) | 0.00000 0.16837 0.50000 |
| F (4g) | 0.00000 0.33308 0.00000 |
| H (4i) | 0.73680 0.00000 0.87176 |
| H (4i) | 0.62798 0.00000 0.23688 |
| H (4i) | 0.26456 0.00000 0.56655 |
| H (4i) | -0.06601 0.00000 0.76577 |
| Li (4g) | 0.00000 0.14999 0.00000 |
| Li (4h) | 0.00000 0.64916 0.50000 |

| $LiFH_3$ | $C2/m$ |
|---|---|
| a, b, c (Å) | 5.471 2.339 4.159 |
| $\alpha, \beta, \gamma$ (Θ) | 90.00 114.91 90.00 |
| F (4i) | 0.12213 0.00000 0.77718 |
| H (4i) | 0.70508 0.00000 0.43205 |
| H (4i) | 0.58171 0.00000 0.44008 |
| H (4i) | 0.46831 0.00000 0.05578 |
| Li (4i) | 0.16968 0.00000 0.19496 |

| $LiF_2H$ | $P\bar{1}$ |
|---|---|
| a, b, c (Å) | 2.072 3.653 5.575 |
| $\alpha, \beta, \gamma$ (Θ) | 93.66 90.84 106.22 |
| F (2i) | 0.08720 0.66367 0.25438 |
| F (2i) | 0.37779 0.23582 0.05694 |
| F (2i) | 0.65682 0.79786 0.58928 |
| H (1f) | 0.50000 0.00000 0.50000 |
| H (2i) | 0.24179 0.46696 0.13467 |
| Li (1g) | 0.00000 0.50000 0.50000 |
| Li (2i) | 0.75520 -0.00428 0.20330 |

| $LiF_2H_2$ | $P\bar{1}$ |
|---|---|
| a, b, c (Å) | 2.094 3.428 4.592 |
| $\alpha, \beta, \gamma$ (Θ) | 73.16 89.61 72.30 |
| F (2i) | 0.65049 0.18534 0.31652 |
| F (2i) | 0.11338 0.26782 -0.09002 |
| H (2i) | -0.02676 0.55265 0.55552 |
| H (2i) | 0.82948 0.27840 0.09284 |
| Li (2i) | 0.64730 0.20067 0.66989 |

| $LiF_3H$ | $P2_1/m$ |
|---|---|
| a, b, c (Å) | 2.089 3.220 5.391 |
| $\alpha, \beta, \gamma$ (Θ) | 90.00 90.71 90.00 |
| F (2e) | 0.51451 0.25000 0.39095 |
| F (2b) | 0.50000 0.00000 0.00000 |
| F (2e) | -0.01554 0.25000 0.71772 |
| H (2e) | 0.24079 0.25000 0.55934 |
| Li (2e) | 0.00561 0.25000 0.17841 |

| $LiF_3H_2$ | $P\bar{1}$ |
|---|---|
| a, b, c (Å) | 2.077 3.583 5.427 |
| $\alpha, \beta, \gamma$ (Θ) | 86.84 89.93 73.77 |
| F (2i) | 0.37143 0.76978 0.05499 |
| F (2i) | 0.06441 0.34009 0.25804 |
| F (2i) | 0.64642 0.22045 0.57852 |
| H (2i) | 0.69023 0.68554 0.55836 |
| H (2i) | 0.24094 0.54177 0.13353 |
| Li (2i) | 0.75306 -0.01152 0.22521 |

| $LiF_3H_3$ | $P1$ |
|---|---|
| a, b, c (Å) | 2.049 3.665 5.827 |
| $\alpha, \beta, \gamma$ (Θ) | 95.96 90.01 106.04 |
| F (1a) | 0.44436 0.33938 0.45558 |
| F (1a) | 0.70794 0.88795 0.54789 |
| F (1a) | 0.12687 0.69697 0.24360 |
| F (1a) | 0.39359 0.22425 0.79348 |
| F (1a) | 0.67218 0.77792 -0.07224 |
| F (1a) | 0.39527 0.21050 0.12328 |
| H (1a) | 0.09037 -0.01379 0.01227 |
| H (1a) | 0.28372 0.67113 0.64680 |
| H (1a) | -0.00066 0.63312 0.74452 |
| H (1a) | 0.05010 0.07190 0.66767 |
| H (1a) | -0.05633 0.47818 0.64161 |
| H (1a) | 0.31629 0.53591 0.35097 |
| Li (1a) | 0.80123 0.04784 0.30580 |
| Li (1a) | 0.01076 0.45030 -0.01220 |

| $LiF_4H$ | $P1$ |
|---|---|
| a, b, c (Å) | 2.082 3.641 6.235 |
| $\alpha, \beta, \gamma$ (Θ) | 88.61 87.95 76.14 |
| F (1a) | 0.00790 0.07062 0.30844 |
| F (1a) | 0.85972 0.03010 0.81682 |
| F (1a) | 0.80534 0.01063 0.10676 |
| F (1a) | 0.58882 0.58352 0.71462 |
| F (1a) | 0.11286 0.44181 -0.02501 |
| F (1a) | 0.31723 0.16796 0.55257 |
| F (1a) | 0.63499 0.61674 0.40776 |
| F (1a) | 0.35680 0.52423 0.18454 |
| H (1a) | 0.69479 0.30561 0.76624 |
| H (1a) | 0.49896 0.37131 0.46904 |
| Li (1a) | 0.44499 0.78721 -0.04925 |
| Li (1a) | -0.00749 0.82499 0.57450 |

| $LiF_4H_4$ | $P1$ |
|---|---|
| a, b, c (Å) | 2.076 3.633 7.400 |
| $\alpha, \beta, \gamma$ (Θ) | 91.90 90.07 106.06 |
| F (1a) | 0.62440 0.26302 0.78869 |
| F (1a) | -0.09958 0.80092 0.67118 |
| F (1a) | 0.32063 0.64643 0.44419 |
| F (1a) | 0.33833 0.72345 -0.09537 |
| F (1a) | 0.64868 0.33835 0.24905 |
| F (1a) | 0.37463 0.78729 0.17190 |
| F (1a) | 0.58491 0.19990 0.52253 |
| F (1a) | 0.06206 0.18603 0.02186 |
| H (1a) | -0.08920 0.05854 0.30278 |
| H (1a) | 0.29125 0.18946 0.88811 |
| H (1a) | 0.15999 0.04744 0.38037 |
| H (1a) | 0.68692 -0.01799 0.58650 |
| H (1a) | -0.00247 0.49513 0.34240 |
| H (1a) | 0.82540 0.87581 0.36613 |
| H (1a) | 0.67573 0.79781 0.80704 |
| H (1a) | 0.27017 0.00232 0.10871 |
| Li (1a) | 0.74785 0.54046 0.04895 |
| Li (1a) | 0.21389 0.44724 0.64565 |

| $Li_2FH$ | $R\overline{3}m$ |
|---|---|
| a, b, c (Å) | 2.154 2.154 18.661 |
| $\alpha, \beta, \gamma$ (Θ) | 90.00 90.00 120.00 |
| F (6c) | 0.00000 0.00000 0.88254 |
| H (6c) | 0.00000 0.00000 0.36587 |
| Li (3b) | 0.00000 0.00000 0.50000 |
| Li (6c) | 0.00000 0.00000 0.26505 |
| Li (3a) | 0.00000 0.00000 0.00000 |

| $Li_2FH_2$ | $Cm$ |
|---|---|
| a, b, c (Å) | 16.966 2.152 3.063 |
| $\alpha, \beta, \gamma$ (Θ) | 90.00 96.08 90.00 |
| F (2a) | 0.18458 0.00000 0.85240 |
| F (2a) | 0.61979 0.00000 0.31435 |
| F (2a) | 0.05218 0.00000 0.77458 |
| F (2a) | 0.75305 0.00000 0.39001 |
| H (2a) | -0.07048 0.00000 0.89713 |
| H (2a) | 0.39171 0.00000 0.66572 |
| H (2a) | -0.07538 0.00000 0.49503 |
| H (2a) | -0.03508 0.00000 0.42285 |
| H (2a) | 0.86107 0.00000 0.21127 |
| H (2a) | -0.03283 0.00000 0.04269 |
| H (2a) | 0.50200 0.00000 0.24106 |
| H (2a) | 0.30262 0.00000 0.87724 |
| Li (2a) | 0.75036 0.00000 0.88897 |
| Li (2a) | 0.48336 0.00000 0.72927 |
| Li (2a) | 0.61809 0.00000 0.81345 |
| Li (2a) | 0.84472 0.00000 0.75399 |
| Li (2a) | 0.18613 0.00000 0.35384 |
| Li (2a) | 0.41382 0.00000 0.18589 |
| Li (2a) | 0.31640 0.00000 0.33134 |
| Li (2a) | 0.05293 0.00000 0.27528 |

| $Li_2F_2H$ | $I4/m$ |
|---|---|
| a, b, c (Å) | 2.196 2.196 27.393 |
| $\alpha, \beta, \gamma$ (Θ) | 90.00 90.00 90.00 |
| F (4e) | 0.00000 0.00000 0.44715 |
| F (4e) | 0.00000 0.00000 0.77846 |
| F (4e) | 0.00000 0.00000 0.66511 |
| F (4e) | 0.00000 0.00000 0.10763 |
| H (8h) | 0.89468 0.36503 0.00000 |
| Li (4e) | 0.00000 0.00000 0.16462 |
| Li (4e) | 0.00000 0.00000 0.39109 |
| Li (4e) | 0.00000 0.00000 0.27823 |
| Li (4e) | 0.00000 0.00000 0.04919 |

| $Li_2F_3H$ | $C2/m$ |
|---|---|
| a, b, c (Å) | 3.696 2.154 5.413 |
| $\alpha, \beta, \gamma$ (Θ) | 90.00 102.26 90.00 |
| F (2c) | 0.00000 0.00000 0.50000 |
| F (4i) | 0.22606 0.00000 0.15209 |
| H (2a) | 0.00000 0.00000 0.00000 |
| Li (4i) | 0.38801 0.00000 0.67543 |

| $Li_3FH$ | $R3m$ |
|---|---|
| a, b, c (Å) | 2.232 2.232 33.566 |
| $\alpha, \beta, \gamma$ (Θ) | 90.00 90.00 120.00 |
| F (3a) | 0.00000 0.00000 0.14201 |
| F (3a) | 0.00000 0.00000 0.86132 |
| F (3a) | 0.00000 0.00000 0.42313 |
| H (3a) | 0.00000 0.00000 0.23982 |
| H (3a) | 0.00000 0.00000 0.60536 |
| H (3a) | 0.00000 0.00000 0.32887 |
| Li (3a) | 0.00000 0.00000 0.78267 |
| Li (3a) | 0.00000 0.00000 0.06551 |
| Li (3a) | 0.00000 0.00000 0.00986 |
| Li (3a) | 0.00000 0.00000 0.37222 |
| Li (3a) | 0.00000 0.00000 -0.07789 |
| Li (3a) | 0.00000 0.00000 0.64636 |
| Li (3a) | 0.00000 0.00000 0.55507 |
| Li (3a) | 0.00000 0.00000 0.50144 |
| Li (3a) | 0.00000 0.00000 0.28707 |

| $Li_3F_2H$ | $P\bar{3}m1$ |
|---|---|
| a, b, c (Å) | 2.157 2.157 4.982 |
| $\alpha, \beta, \gamma$ (Θ) | 90.00 90.00 120.00 |
| F (2d) | 0.33333 0.66667 0.31597 |
| H (1a) | 0.00000 0.00000 0.00000 |
| Li (2d) | 0.33333 0.66667 0.86695 |
| Li (1b) | 0.00000 0.00000 0.50000 |

| $Li_3F_3H$ | $P\bar{1}$ |
|---|---|
| a, b, c (Å) | 3.116 3.784 8.987 |
| $\alpha, \beta, \gamma$ (Θ) | 92.53 92.93 113.81 |
| F (2i) | 0.89127 0.85119 0.22699 |
| F (2i) | 0.47574 -0.07957 0.61618 |
| F (2i) | 0.79915 0.53602 0.69472 |
| F (2i) | 0.26568 0.61229 0.07771 |
| F (2i) | 0.56109 0.24494 0.15156 |
| F (2i) | 0.84034 0.69386 0.46137 |
| H (2i) | 0.35125 0.01461 -0.04397 |
| H (2i) | 0.16668 -0.00785 0.00000 |
| Li (2i) | 0.60776 0.14566 0.77129 |
| Li (2i) | -0.02393 -0.07889 0.61699 |
| Li (2i) | 0.05351 0.22746 0.14785 |
| Li (2i) | 0.29742 0.53289 0.69351 |
| Li (2i) | 0.77873 0.63892 0.06836 |
| Li (2i) | 0.33930 0.69214 0.46075 |

| $Li_3F_4H$ | $C2/m$ |
|---|---|
| a, b, c (Å) | 3.723 2.164 7.214 |
| $\alpha, \beta, \gamma$ (Θ) | 90.00 100.59 90.00 |
| F (4i) | 0.63850 0.00000 0.88708 |
| F (4i) | 0.21200 0.00000 0.62964 |
| H (2b) | 0.00000 0.50000 0.00000 |
| Li (2d) | 0.00000 0.50000 0.50000 |
| Li (4i) | -0.07490 0.00000 0.75951 |

| $Li_4FH_4$ | $P1$ |
|---|---|
| a, b, c (Å) | 2.314 3.711 8.633 |
| $\alpha, \beta, \gamma$ (Θ) | 91.13 90.10 108.14 |
| F (1a) | 0.59170 0.33681 0.26041 |
| F (1a) | 0.85907 0.87258 0.15615 |
| F (1a) | 0.32254 0.79694 0.36085 |
| H (1a) | 0.33954 0.83394 -0.01460 |
| H (1a) | 0.00624 0.48039 0.88868 |
| H (1a) | 0.86435 0.87818 0.52901 |
| H (1a) | -0.02724 0.09598 0.78595 |
| H (1a) | 0.64160 0.43183 0.59121 |
| H (1a) | 0.42512 -0.00164 0.66205 |
| H (1a) | 0.10891 0.37658 0.06529 |
| H (1a) | 0.54455 0.24194 -0.08058 |
| H (1a) | 0.77082 0.69222 0.85236 |
| H (1a) | 0.07762 0.30571 0.45327 |
| H (1a) | 0.30642 0.44107 0.89172 |
| H (1a) | 0.20316 0.55145 0.71558 |
| Li (1a) | 0.69535 0.54169 0.41940 |
| Li (1a) | -0.03931 0.07684 -0.04682 |
| Li (1a) | -0.03721 0.07807 0.31738 |
| Li (1a) | 0.81295 0.77437 0.68749 |
| Li (1a) | 0.25204 0.65359 0.55441 |
| Li (1a) | 0.35493 0.85918 0.82815 |
| Li (1a) | 0.03296 0.21383 0.62440 |
| Li (1a) | 0.47532 0.10042 0.49303 |
| Li (1a) | 0.71543 0.59225 0.01266 |
| Li (1a) | 0.59673 0.33710 0.76473 |
| Li (1a) | 0.21931 0.59289 0.19648 |
| Li (1a) | 0.48951 0.13433 0.09955 |

| $Li_4F_3H$ | $R\bar{3}m$ |
|---|---|
| a, b, c (Å) | 2.170 2.170 20.286 |
| $\alpha, \beta, \gamma$ (Θ) | 90.00 90.00 120.00 |
| F (3a) | 0.00000 0.00000 0.00000 |
| F (6c) | 0.00000 0.00000 0.24353 |
| H (3b) | 0.00000 0.00000 0.50000 |
| Li (6c) | 0.00000 0.00000 0.86565 |
| Li (6c) | 0.00000 0.00000 0.62168 |

| $Li_4F_4H$ | $P\bar{1}$ |
|---|---|
| a, b, c (Å) | 3.114 4.894 8.453 |
| $\alpha, \beta, \gamma$ (Θ) | 86.43 80.15 88.47 |
| F (2i) | 0.31539 0.26544 0.84843 |
| F (2i) | 0.38078 0.67354 0.73193 |
| F (2i) | 0.43547 0.08706 0.61496 |
| F (2i) | 0.11648 0.62006 0.32027 |
| F (2i) | 0.20850 0.44148 0.08735 |
| F (2i) | 0.15307 0.03179 0.20491 |
| F (2i) | 0.26626 0.85300 -0.03110 |
| F (2i) | -0.01137 0.79898 0.56028 |
| H (2i) | 0.32556 0.51342 0.49745 |
| H (2i) | 0.14512 0.43119 0.51972 |
| Li (2i) | 0.34845 -0.03076 0.79164 |
| Li (2i) | 0.39094 0.38710 0.66521 |
| Li (2i) | 0.23568 0.14835 0.02668 |
| Li (2i) | 0.18744 0.73743 0.14504 |
| Li (2i) | 0.70705 0.44207 0.09020 |
| Li (2i) | 0.06725 -0.09001 0.38156 |
| Li (2i) | 0.50878 0.22228 0.44434 |
| Li (2i) | 0.12055 0.32552 0.26505 |

| $LiF_4H_3$ | $P\bar{1}$ |
|---|---|
| a, b, c (Å) | 2.062 3.552 7.265 |
| $\alpha, \beta, \gamma$ (Θ) | 87.70 82.21 73.40 |
| F (2i) | 0.48987 0.67192 0.81783 |
| F (2i) | 0.83726 0.13266 0.70393 |
| F (2i) | 0.17367 0.22396 -0.05307 |
| F (2i) | 0.60830 0.72985 0.54251 |
| H (2i) | 0.78497 0.44154 0.89593 |
| H (2i) | 0.66002 0.03115 0.13703 |
| H (2i) | 0.73012 -0.04426 0.60384 |
| Li (2i) | 0.18090 0.47762 0.66028 |

## S6 Structural Coordinates of the Reference Phases at 300 GPa

| Li | $P4_2/mbc$ |
|---|---|
| a, b, c (Å) | 3.674 3.674 4.496 |
| $\alpha, \beta, \gamma$ (Θ) | 90.00 90.00 90.00 |
| Li (8h) | 0.67131 0.55874 0.00000 |
| Li (8g) | 0.63256 0.13256 0.25000 |

| F | $Cmca$ |
|---|---|
| a, b, c (Å) | 3.320 2.251 5.029 |
| $\alpha, \beta, \gamma$ (Θ) | 90.00 90.00 90.00 |
| F (8f) | 0.00000 0.33740 0.38212 |

| H | $Cmca$ |
|---|---|
| a, b, c (Å) | 2.558 4.754 2.870 |
| $\alpha, \beta, \gamma$ (Θ) | 90.00 90.00 90.00 |
| H (8f) | 0.00000 0.50367 0.36507 |
| H (8f) | 0.00000 0.63183 0.04606 |
| H (8f) | 0.00000 0.76774 0.18308 |

| LiF | $Fm\bar{3}m$ |
|---|---|
| a, b, c (Å) | 3.114 3.114 3.114 |
| $\alpha, \beta, \gamma$ (Θ) | 90.00 90.00 90.00 |
| F (4b) | 0.50000 0.50000 0.50000 |
| Li (4a) | 0.00000 0.00000 0.00000 |

| HF | $Pnma$ |
|---|---|
| a, b, c (Å) | 3.488 3.317 2.057 |
| $\alpha, \beta, \gamma$ (Θ) | 90.00 90.00 90.00 |
| F (4c) | 0.66775 0.25000 0.03138 |
| H (4c) | 0.42470 0.25000 0.73253 |

| LiH | $Pm\bar{3}m$ |
|---|---|
| a, b, c (Å) | 1.686 1.686 1.686 |
| $\alpha, \beta, \gamma$ (Θ) | 90.00 90.00 90.00 |
| H (1b) | 0.50000 0.50000 0.50000 |
| Li (1a) | 0.00000 0.00000 0.00000 |

| $LiH_2$ | $P4/mbm$ |
|---|---|
| a, b, c (Å) | 3.740 3.740 1.802 |
| $\alpha, \beta, \gamma$ (Θ) | 90.00 90.00 90.00 |
| H (4g) | 0.64753 0.14753 0.00000 |
| H (4e) | 0.00000 0.00000 0.70547 |
| Li (4h) | 0.84526 0.34526 0.50000 |

| $LiH_6$ | $R\bar{3}m$ |
|---|---|
| a, b, c (Å) | 2.859 2.859 5.018 |
| $\alpha, \beta, \gamma$ (Θ) | 90.00 90.00 120.00 |
| H (18h) | 0.16456 0.83544 0.25053 |
| Li (3a) | 0.00000 0.00000 0.00000 |

# S7 Bader Analysis at 300 GPa

Table S3: Bader charges for F, H and Li atoms and the overall charges of the $(F_a\text{-}H_a\text{-}F_b)^-$ (top seven rows) and $(F_aH_a\text{-}F_{\text{middle}}\text{-}H_bF_b)^-$ motifs in the studied systems (bottom two rows). In the asymmetric anions, $F_a/F_b$ represent the Bader charges of the F atoms that are closer/farther to the nearest H atoms, respectively. $Li_a/Li_b/Li_{\text{middle}}$ are the nearest Li atoms to $F_a/F_b/F_{\text{middle}}$.

| System | $F_a$ ($e$) | $F_b$ ($e$) | $H_a$ ($e$) | $H_b$ ($e$) | $Li_a$ ($e$) | $Li_b$ ($e$) | $Li_{\text{middle}}$ ($e$) | $F_{\text{middle}}$ ($e$) | $H_nF_{n+1}^-$ |
|---|---|---|---|---|---|---|---|---|---|
| HF | −0.75 | −0.75 | +0.75 | – | – | – | – | – | – |
| $LiF_2H$[a] | −0.79 | −0.79 | +0.73 | – | +0.83 | +0.83 | – | – | −0.85 |
| $LiF_2H$[a] | −0.80 | −0.79 | +0.74 | – | +0.85 | +0.85 | – | −0.85 | |
| $Li_3F_4H$ | −0.79 | −0.79 | +0.75 | – | +0.83 | +0.83 | – | – | −0.83 |
| $LiF_4H_4$ | −0.74 | −0.75 | +0.73 | – | +0.86 | +0.86 | – | – | −0.76 |
| $Li_2F_3H$ | −0.79 | −0.79 | +0.75 | – | +0.83 | +0.83 | – | – | −0.83 |
| $LiF_3H$ | −0.63 | −0.65 | +0.76 | – | +0.85 | +0.85 | – | – | −0.52 |
| $LiF_3H_2$ | −0.79 | −0.79 | +0.75 | +0.75 | +0.86 | +0.86 | +0.86 | −0.77 | −0.85 |
| $LiF_4H_4$ | −0.78 | −0.79 | +0.75 | +0.75 | +0.86 | +0.86 | +0.86 | −0.77 | −0.84 |

[a] Linear and bent bifluoride anions are present in this phase.

## S8 Electron Localization Function (ELF) Calculated for $LiF_3H_2$, $LiF_2H$ and $LiF_4H_4$

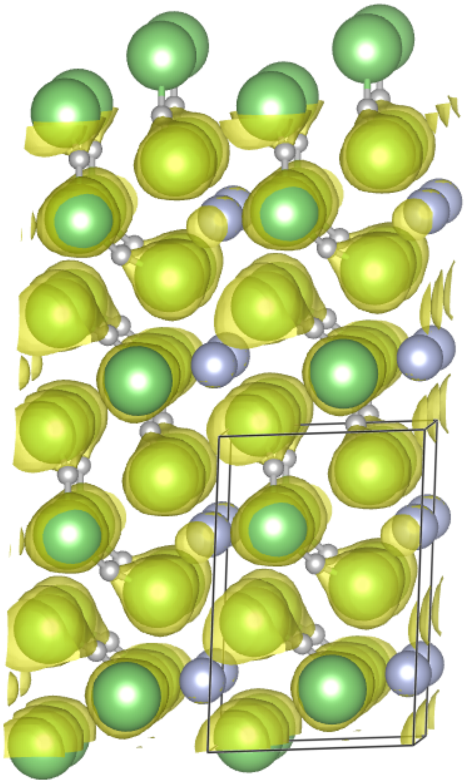

Figure S6: The isosurface (ELF=0.7) of the electron localization function of $LiF_3H_2$ at 300 GPa. Li/F/H are colored blue/green/white.

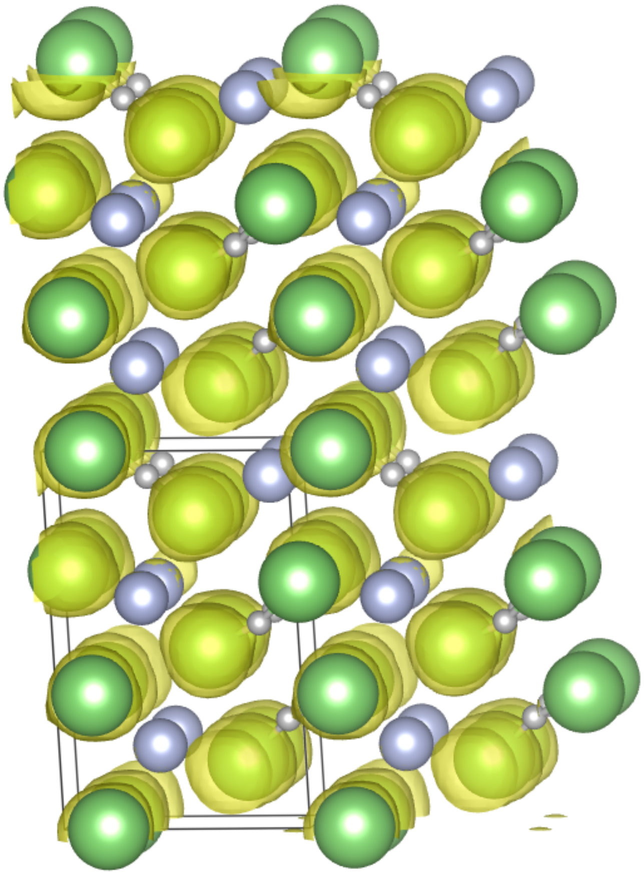

Figure S7: The isosurface (ELF=0.7) of the electron localization function of $LiF_2H$ at 300 GPa. Li/F/H are colored blue/green/white.

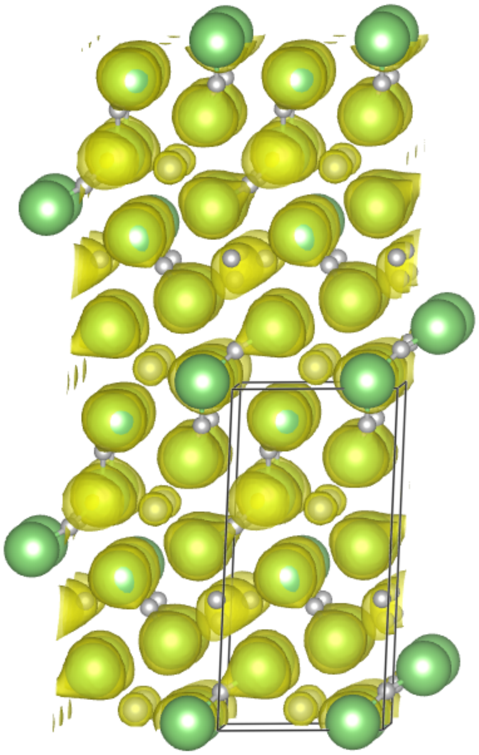

Figure S8: The isosurface (ELF=0.7) of the electron localization function of $LiF_4H_4$ at 300 GPa. Li/F/H are colored blue/green/white.

# S9 Phonon DOS of Li-F-H Phases at 300 GPa

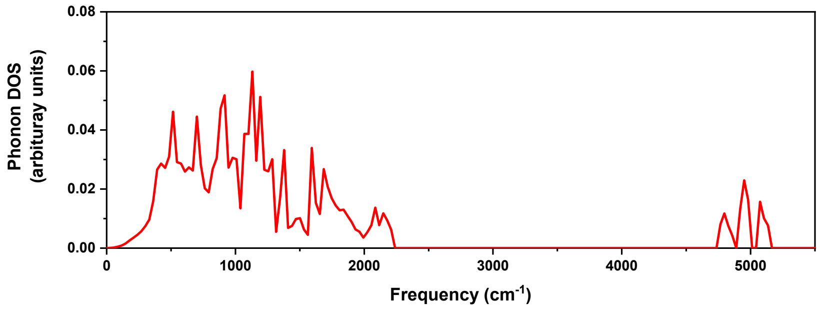


Figure S9: Phonon density of states of the $LiFH_2$ phase.

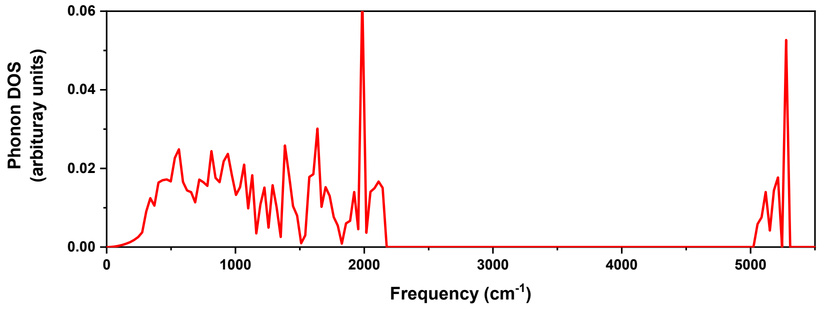


Figure S10: Phonon density of states of the $LiFH_3$ phase.

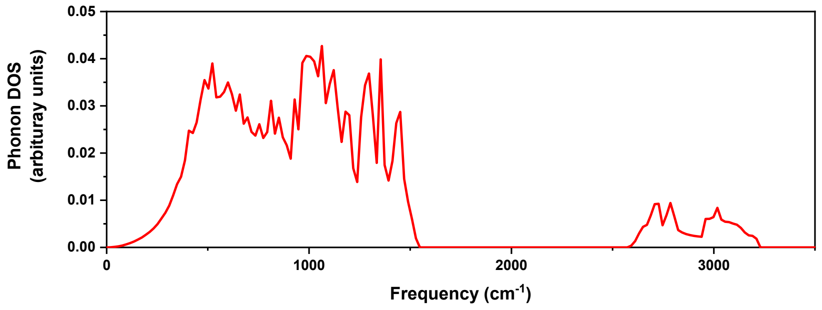


Figure S11: Phonon density of states of the $LiF_2H$ phase.

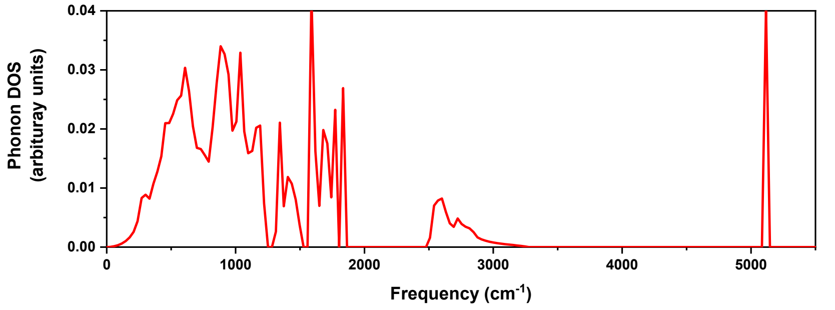


Figure S12: Phonon density of states of the $LiF_2H_2$ phase.

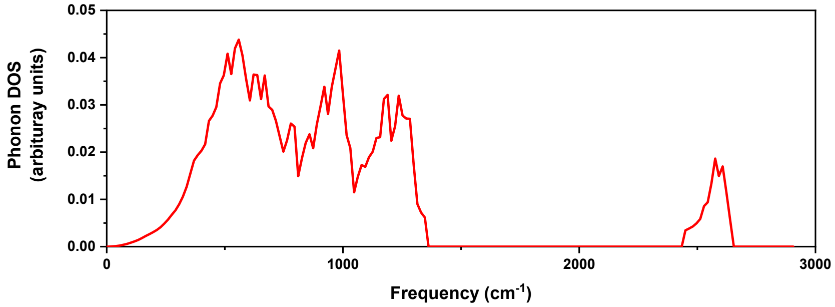


Figure S13: Phonon density of states of the $LiF_3H$ phase.

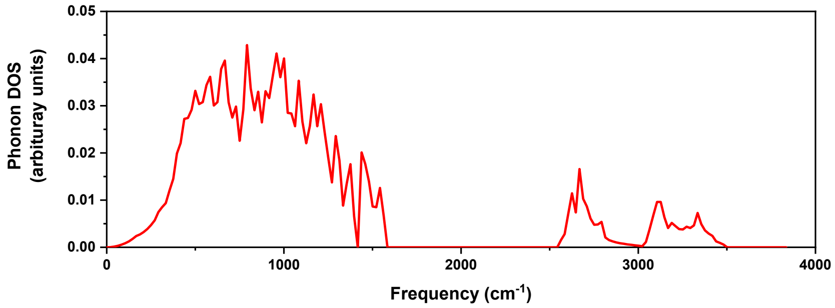


Figure S14: Phonon density of states of the $LiF_3H_2$ phase.

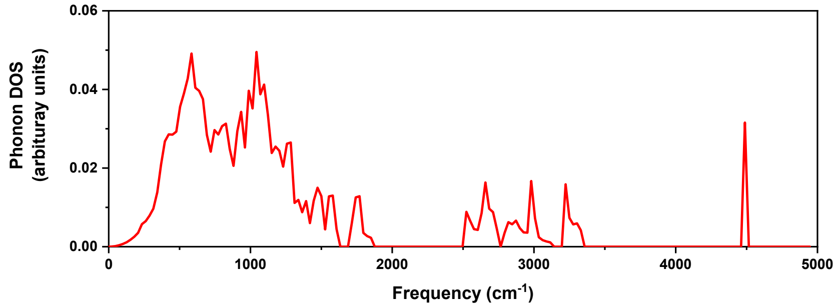


Figure S15: Phonon density of states of the $LiF_3H_3$ phase.

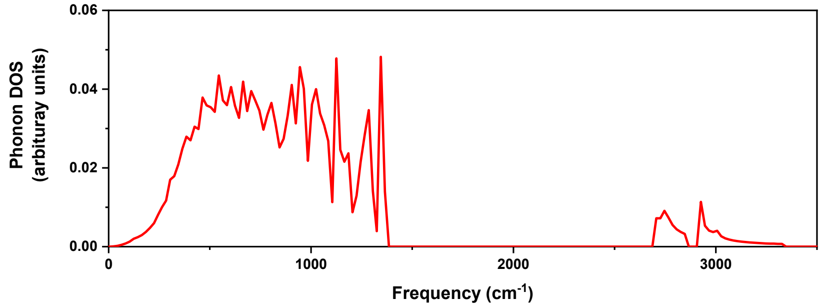


Figure S16: Phonon density of states of the $LiF_4H$ phase.

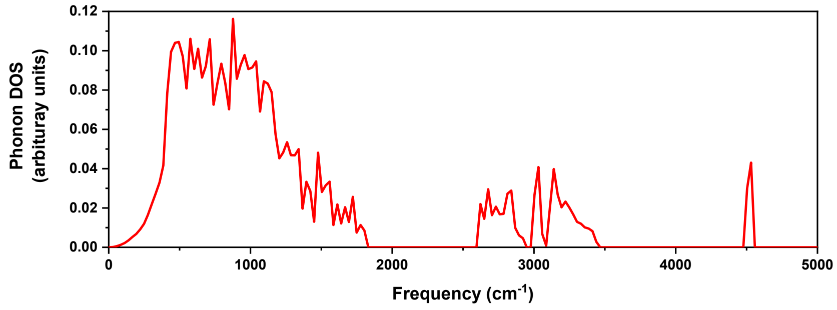


Figure S17: Phonon density of states of the $LiF_4H_4$ phase.

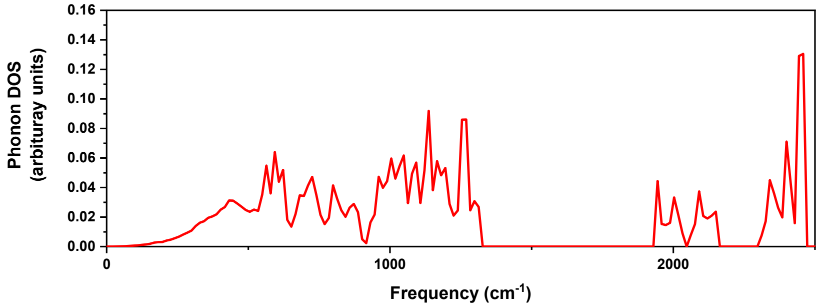


Figure S18: Phonon density of states of the $Li_2FH$ phase.

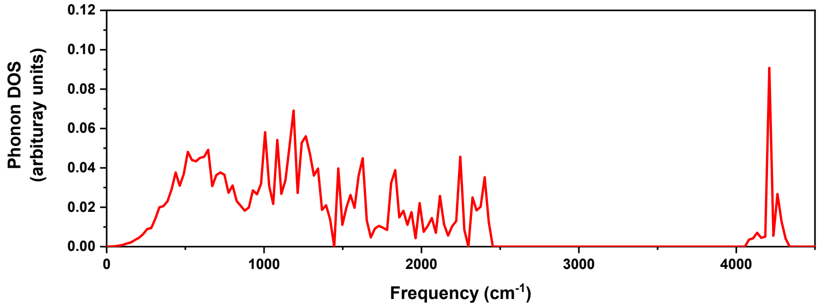


Figure S19: Phonon density of states of the $Li_2FH_2$ phase.

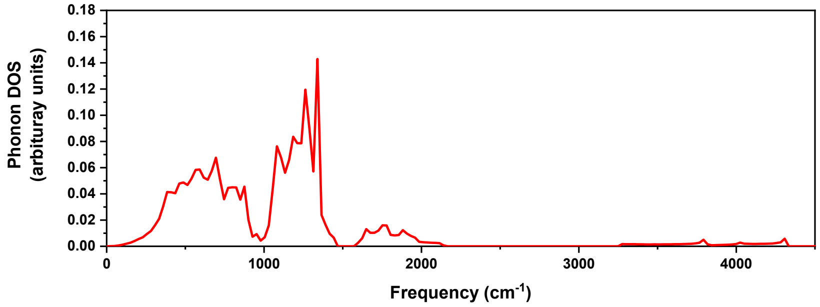


Figure S20: Phonon density of states of the $Li_2F_2H$ phase.

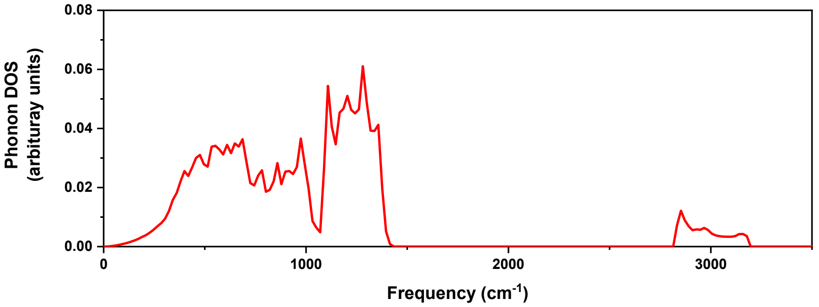


Figure S21: Phonon density of states of the $Li_2F_3H$ phase.

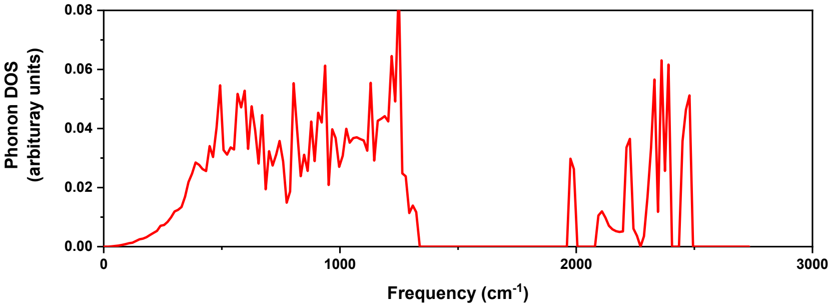


Figure S22: Phonon density of states of the $Li_3FH$ phase.

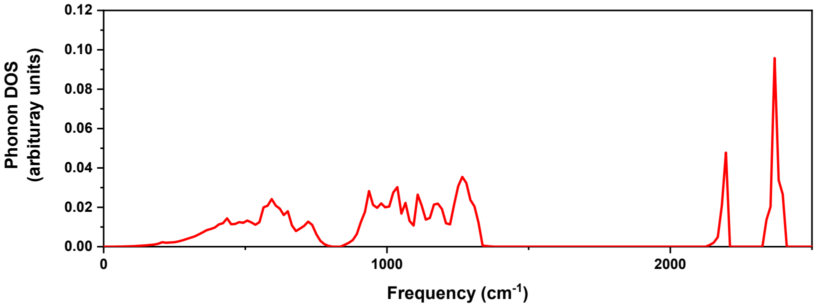


Figure S23: Phonon density of states of the $Li_3F_2H$ phase.

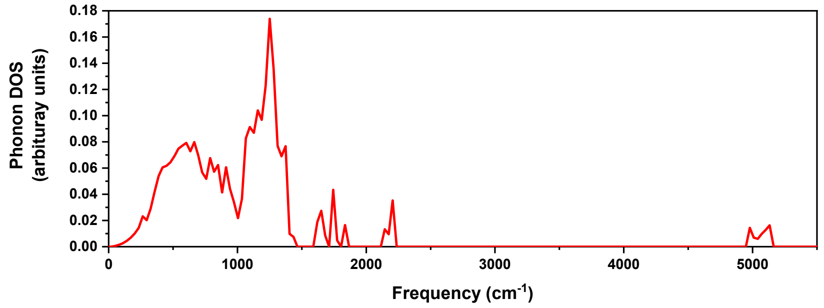


Figure S24: Phonon density of states of the $Li_3F_3H$ phase.

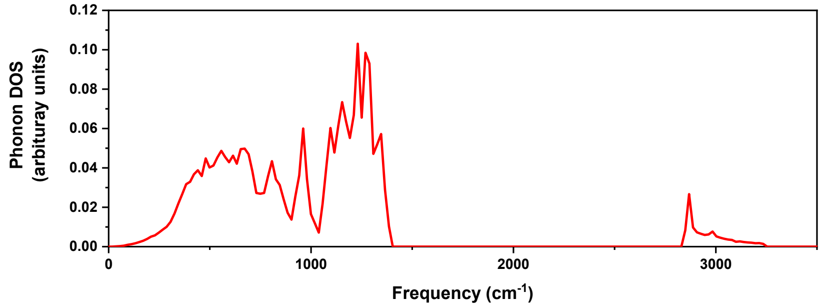


Figure S25: Phonon density of states of the $Li_3F_4H$ phase.

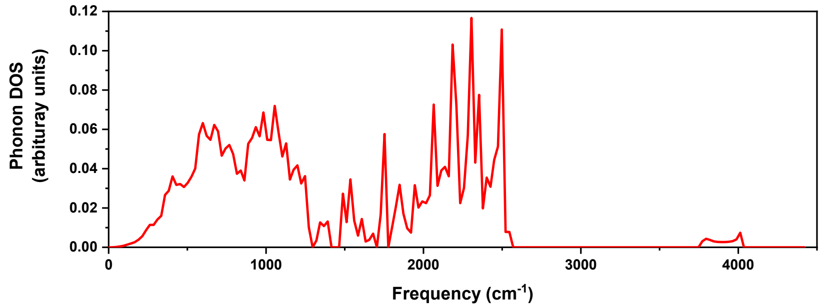


Figure S26: Phonon density of states of the $Li_4FH_4$ phase.

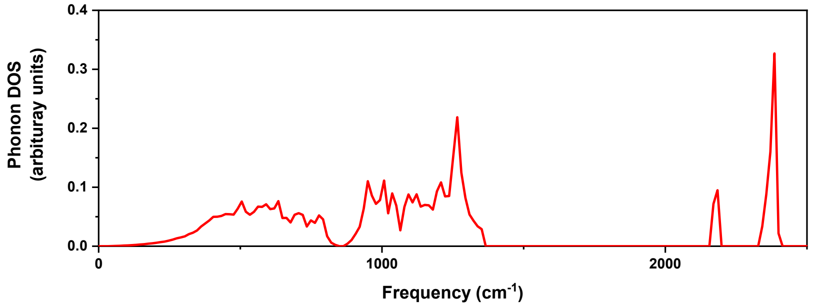


Figure S27: Phonon density of states of the $Li_4F_3H$ phase.

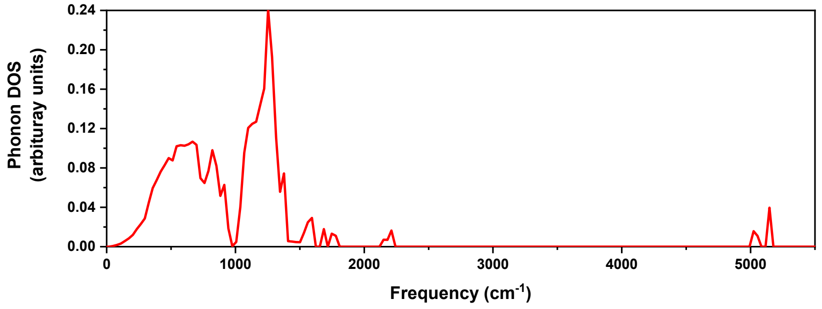


Figure S28: Phonon density of states of the $Li_4F_4H$ phase.

## S10 Infrared (IR) Spectra of HF and Li-F-H Phases at 300 GPa

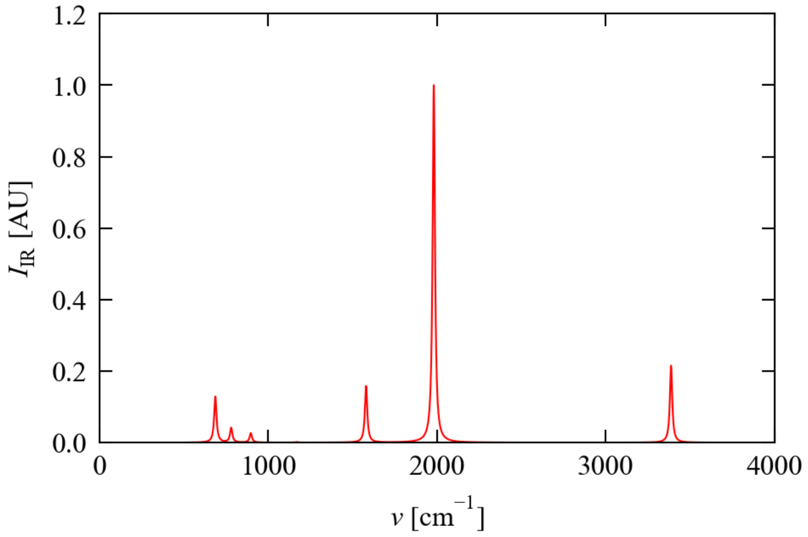


Figure S29: Infrared (IR) spectrum of the HF phase at 300 GPa.

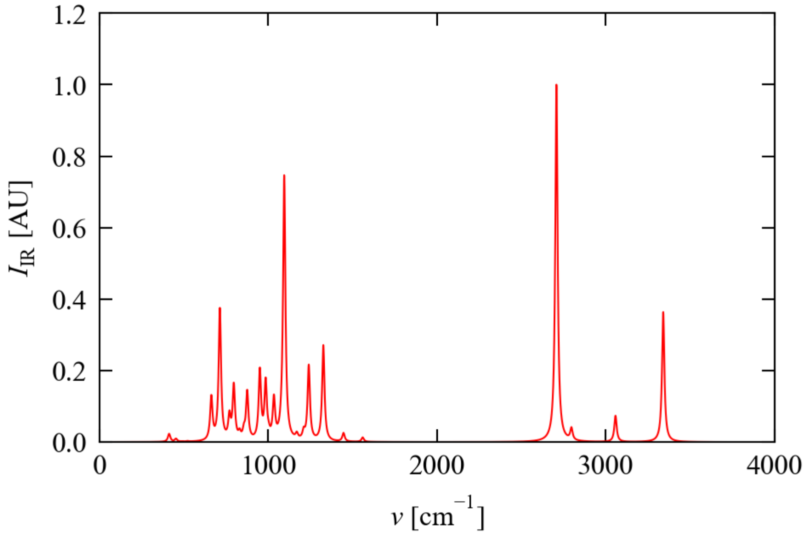


Figure S30: Infrared (IR) spectrum of the $LiF_3H_2$ phase at 300 GPa.

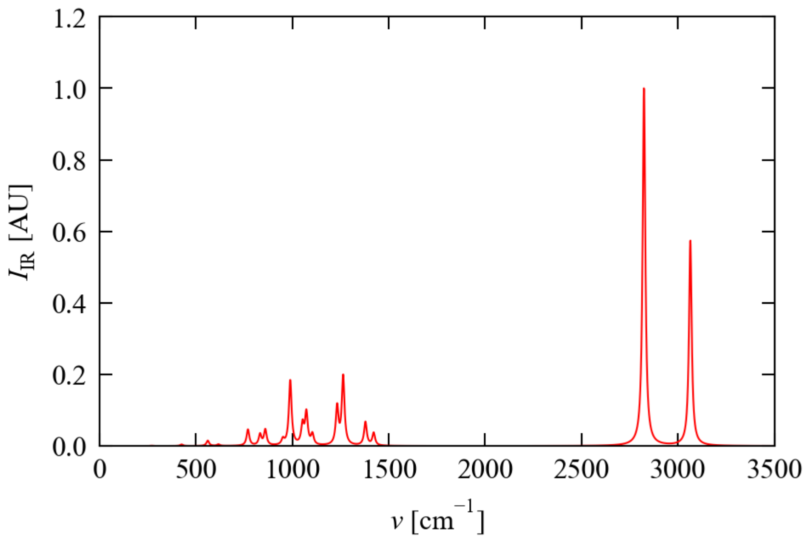


Figure S31: Infrared (IR) spectrum of the $LiF_2H$ phase at 300 GPa.

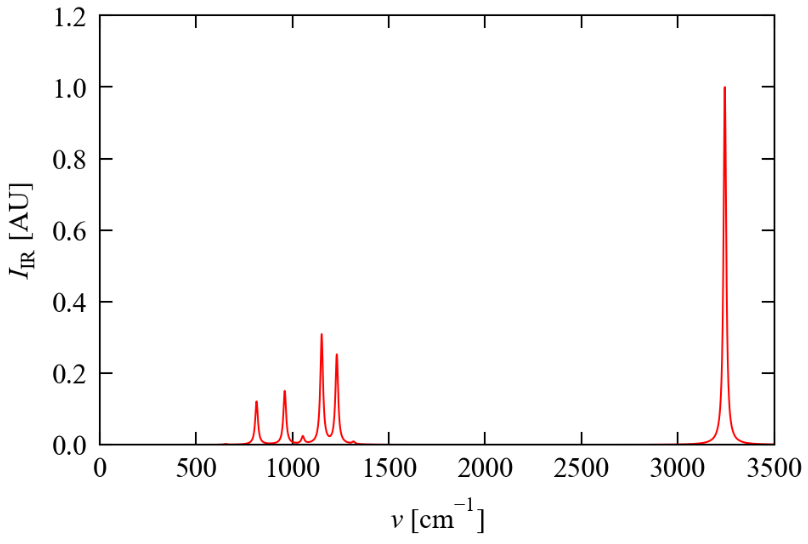


Figure S32: Infrared (IR) spectrum of the $Li_3F_4H$ phase at 300 GPa.

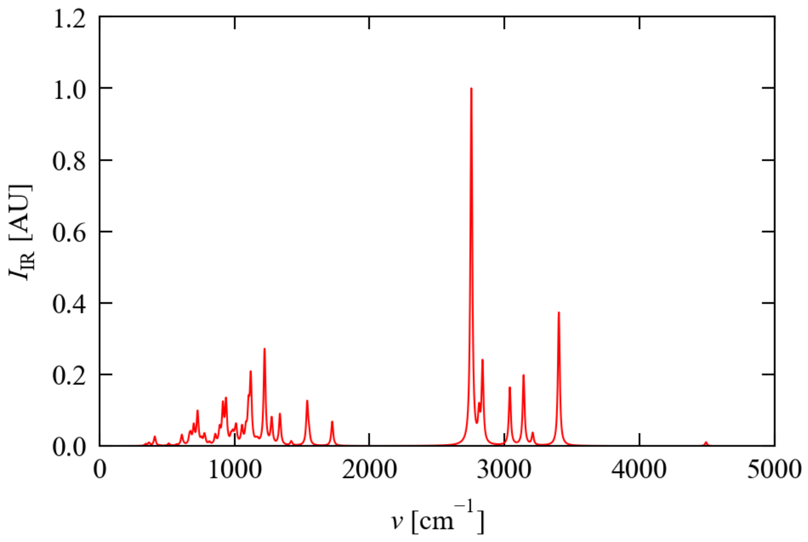


Figure S33: Infrared (IR) spectrum of the $LiF_4H_4$ phase at 300 GPa.

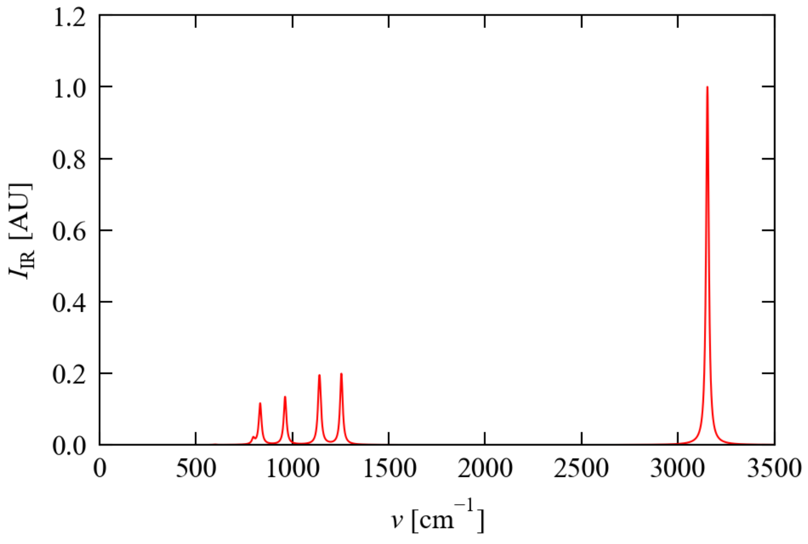


Figure S34: Infrared (IR) spectrum of the $Li_2F_3H$ phase at 300 GPa.

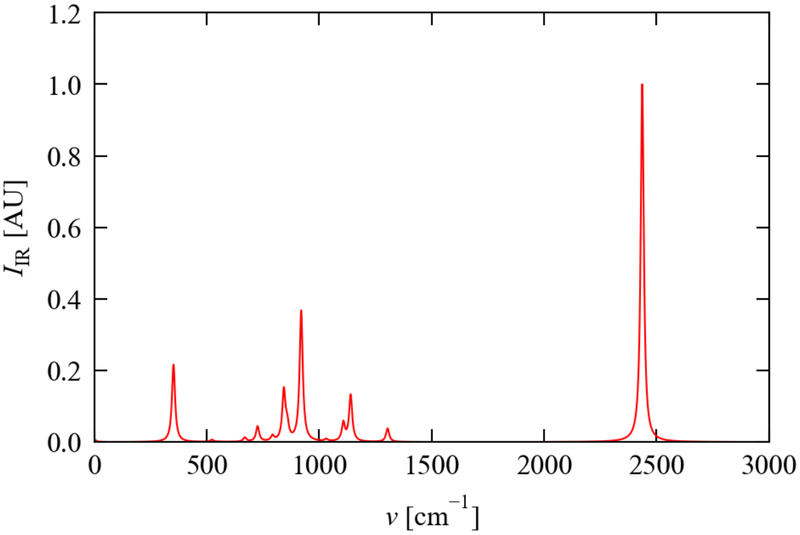


Figure S35: Infrared (IR) spectrum of the $LiF_3H$ phase at 300 GPa.

# References


[1] J. Lv, Y. Wang, L. Zhu, Y. Ma, *Phys. Rev. Lett.* **2011**, *106*, 015503.

[2] C. J. Pickard, R. J. Needs, *Nat. Phys.* **2007**, *3*, 473–476.

[3] M. A. Olson, S. Bhatia, P. Larson, B. Militzer, *J. Chem. Phys.* **2020**, *153*, 094111.

[4] N. A. Smirnov, *Phys. Rev. B* **2011**, *83*, 014109.

[5] Z.-H. Sun, J. Dong, Y.-W. Xia, *Physica B* **2011**, *406*, 3660–3665.

[6] D. Duan, X. Huang, F. Tian, Y. Liu, D. Li, H. Yu, B. Liu, W. Tian, T. Cui, *J. Phys. Chem. A* **2015**, *119*, 11059–11065.

[7] L. Zhang, Y. Wang, X. Zhang, Y. Ma, *Phys. Rev. B* **2010**, *82*, 014108.

[8] Z. Wang, H. Cui, J. Hou, X. Dong, *Geosci. Front.* **2020**.

[9] M. J. Van Setten, V. A. Popa, G. A. De Wijs, G. Brocks, *Phys. Rev. B* **2007**, *75*, 035204.

[10] E. Zurek, R. Hoffmann, N. Ashcroft, A. R. Oganov, A. O. Lyakhov, *Proc. Natl. Acad. Sci. U.S.A.* **2009**, *106*, 17640–17643.

[11] J. J. Gilman, *Phys. Rev. Lett.* **1971**, *26*, 546.
